# Supplementary material for: Towards Communication-Efficient and Privacy-Preserving Federated Representation Learning
Source: arXiv:2109.14611 source file (2022-01-15)
Supplement: Supplementary file 1 [file appendix.tex]

\newpage
\begin{figure*}[p]
    \centering
    \begin{subfigure}[CIFAR10]{
        \begin{minipage}{\textwidth}
            \includegraphics[width=1\textwidth]{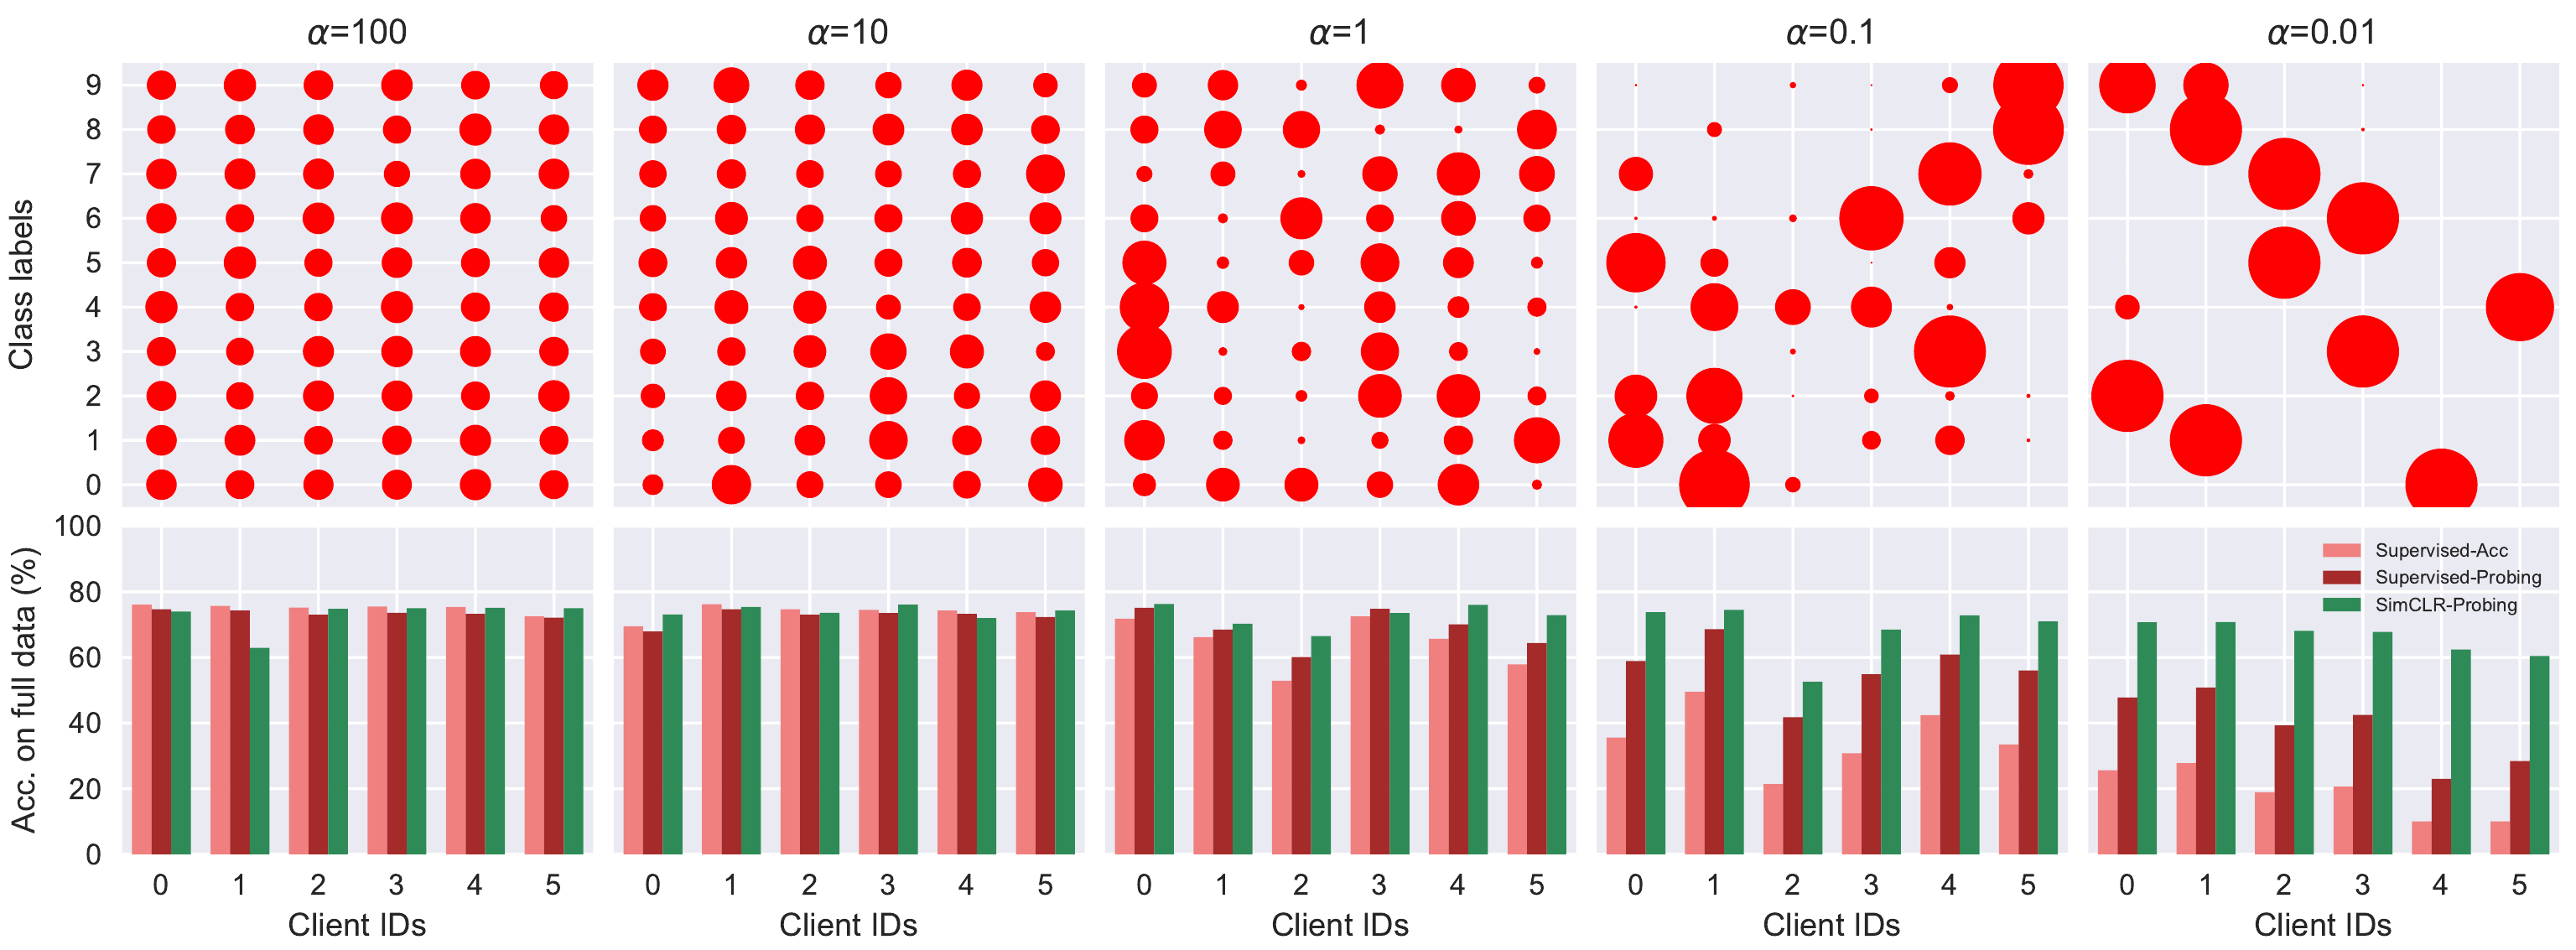}
        \end{minipage}
    }
    \end{subfigure}
    \hfill
    \begin{subfigure}[CIFAR100]{
        \begin{minipage}{\textwidth}
            \includegraphics[width=1\textwidth]{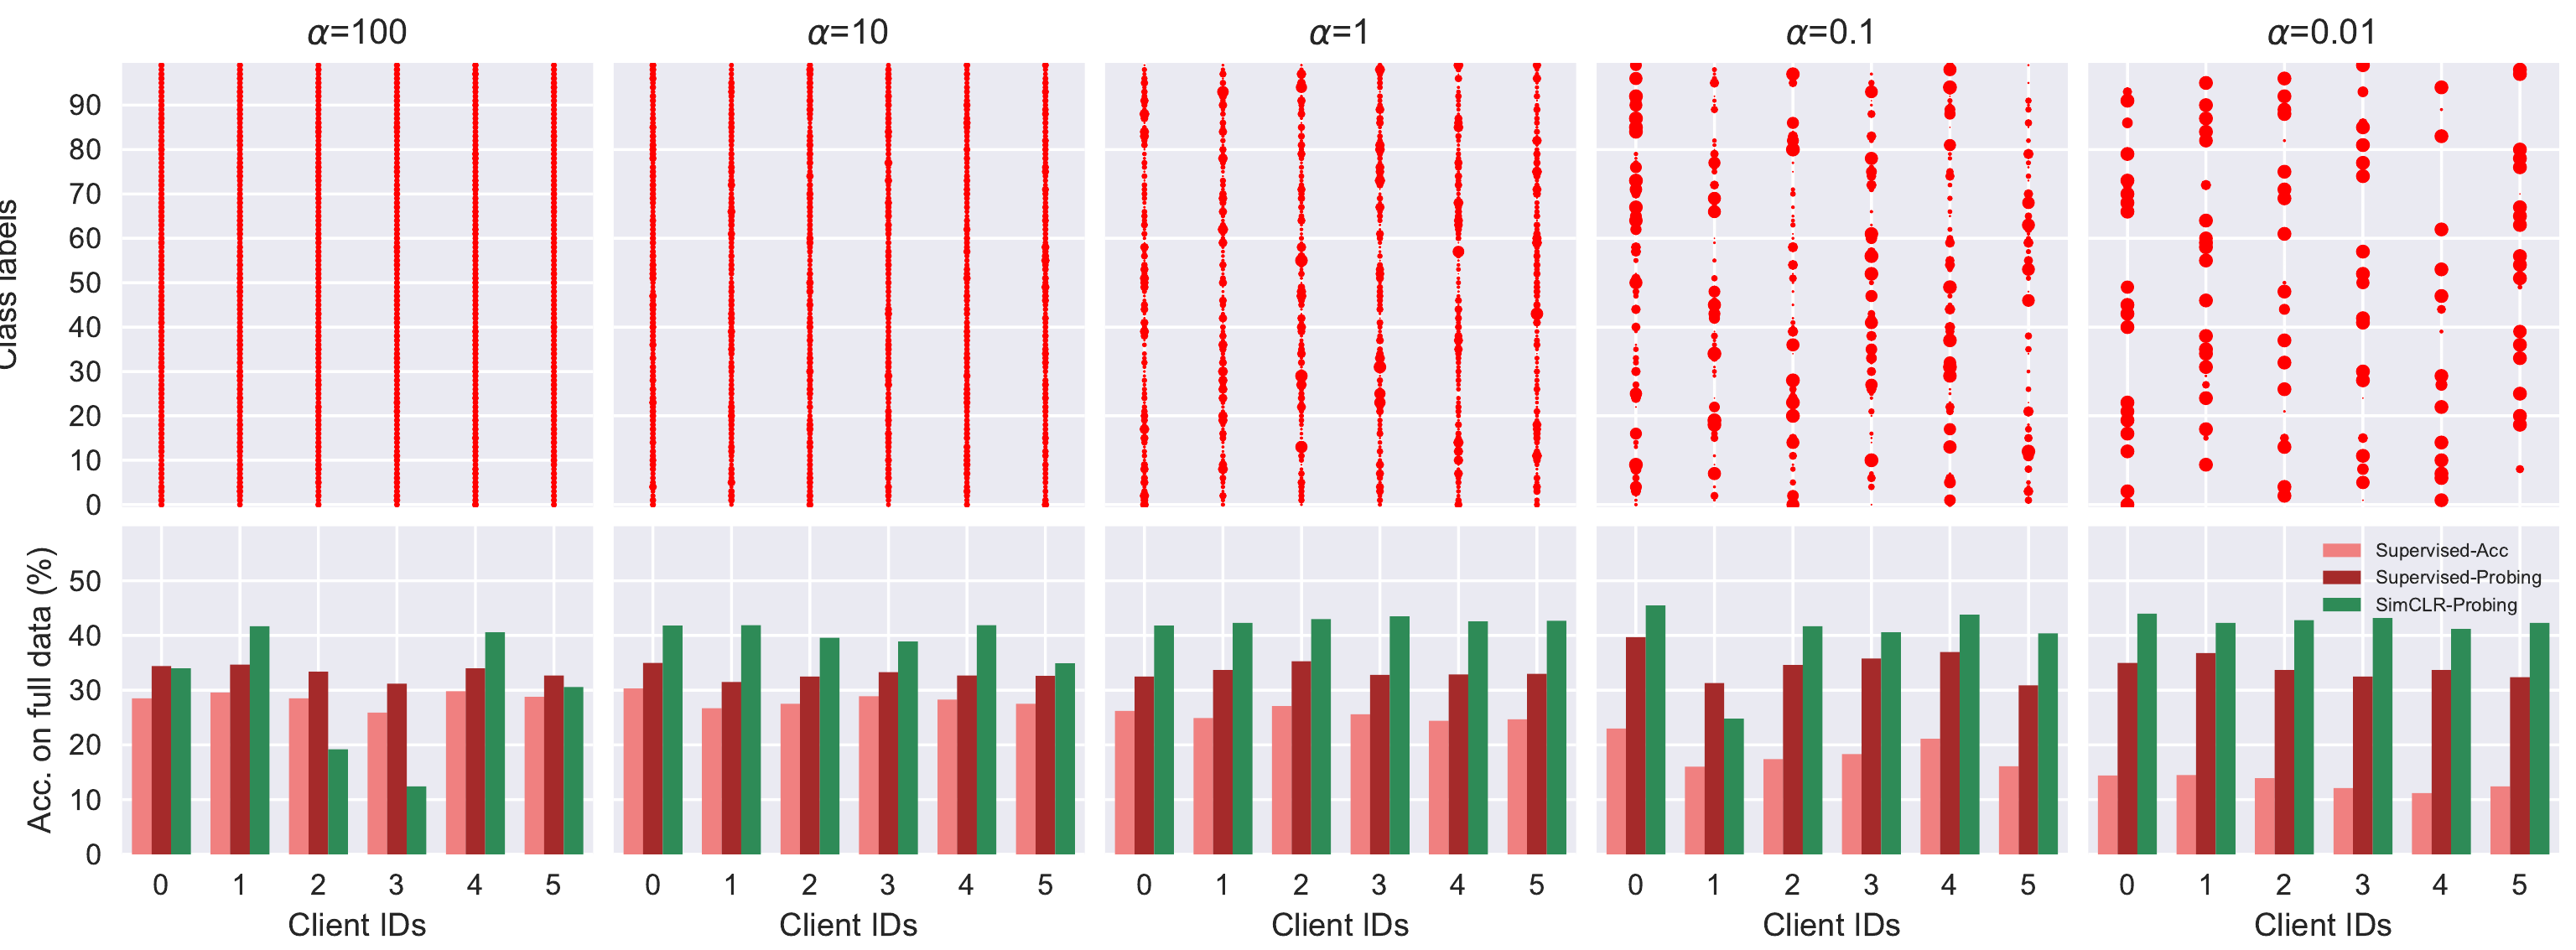}
        \end{minipage}
    }
    \end{subfigure}
    \caption{Local training of supervised and self-supervised learning on CIFAR10/100. The top row of both subfigures visualizes the non-\iid-ness of the data distribution; the radius of each circle represents the size of the local dataset. The bottom row compares the behavior of supervised and self-supervised local training. The self-supervised framework SimCLR is more robust than the supervised method. For CIFAR10, the performance deterioration happens especially at $\alpha$=0.01 for supervised learning paradigm, where client No.4 and No.5 hold only single category of the data. This phenomenon, however, is not apparent in CIFAR100 since the number of semantic classes significantly surpasses the number of the clients and the situation of one client holding single dangling class doesn't occur.}
    \label{fig:obs-full}
\end{figure*}

%%%%%%%%%%%%%%%%%% CIFAR10.%%%%%%%%%%%%%%%%%%%
%%%%%%%%%%%%%%%%%% SL Local Acc. %%%%%%%%%%%%%
\begin{table*}[p]
\vspace{5em}
\begin{center}
\tablestyle{7.5pt}{1.35}
\begin{tabular}{c|c|c|c|cccccc|cc}
\multirow{2}{*}{\textbf{Dataset}} & \multirow{2}{*}{\textbf{Method}} & \multirow{2}{*}{\textbf{Evaluation}} & \multirow{2}{*}{\textbf{Non-i.i.d-ness $\alpha$}} & \multicolumn{6}{c|}{\textbf{Client ID}} & \multirow{2}{*}{\textbf{Mean}} & \multirow{2}{*}{\textbf{Min}} \\
& & & & C0   & C1   & C2   & C3   & C4   & C5 \\
\shline
\multirow{15}{*}{CIFAR10} & \multirow{10}{*}{Supervised} & \multirow{5}{*}{Acc.} & 100 & 76.1 & 75.7 & 75.2 & 75.5 & 75.4 & 72.5 & 75.1 & 72.5 \\
& & & 10                   & 69.5 & 76.2 & 74.7 & 74.5 & 74.3 & 73.8 & 73.8 & 69.5 \\
& & & 1                    & 71.8 & 66.2 & 52.9 & 72.5 & 65.7 & 57.9 & 64.5 & 52.9 \\
& & & 0.1                  & 35.6 & 49.5 & 21.4 & 30.8 & 42.4 & 33.5 & 35.5 & 21.4 \\
& & & 0.01                 & 25.6 & 27.8 & 18.9 & 20.6 & 10.0 & 10.0 & 18.8 & 10.0 \\
\cline{3-12}
&  & \multirow{5}{*}{\shortstack{Linear\\ Probe}} & 100 & 74.7 & 74.3 & 73.0 & 73.6 & 73.3 & 72.1 & 73.5 & 72.1 \\
& & & 10                   & 67.9 & 74.7 & 73.0 & 73.5 & 73.3 & 72.3 & 72.5 & 67.9 \\
& & & 1                    & 75.1 & 68.5 & 60.1 & 74.8 & 70.1 & 64.4 & 68.8 & 60.1 \\
& & & 0.1                  & 58.9 & 68.6 & 41.8 & 54.9 & 60.9 & 56.0 & 56.9 & 41.8 \\
& & & 0.01                 & 47.8 & 50.8 & 39.3 & 42.5 & 23.0 & 28.4 & 38.6 & 23.0 \\
\cline{2-12}
& \multirow{5}{*}{SimCLR} & \multirow{5}{*}{\shortstack{Linear\\ Probe}} & 100 & 74.0 & 62.9 & 74.8 & 75.0 & 75.1 & 75.0 & 72.8    & 62.9 \\
& & & 10                     & 73.1 & 75.4 & 73.6 & 76.1 & 72.0 & 74.3 & 74.1    & 72.0 \\
& & & 1                      & 76.3 & 70.3 & 66.5 & 73.5 & 76.0 & 72.9 & 72.6    & 66.5 \\
& & & 0.1                    & 73.8 & 74.5 & 52.6 & 68.5 & 72.8 & 71.0 & 68.9    & 52.6 \\
& & & 0.01                   & 70.7 & 70.8 & 68.1 & 67.8 & 62.4 & 60.4 & 66.7    & 60.4 \\
\shline
\multirow{15}{*}{CIFAR100} & \multirow{10}{*}{Supervised} & \multirow{5}{*}{Acc.} & 100 & 28.5 & 29.6 & 28.5 & 25.9 & 29.8 & 28.8 & 28.5    & 25.9 \\
& & & 10                   & 30.3 & 26.7 & 27.5 & 28.9 & 28.3 & 27.5 & 28.2    & 26.7 \\
& & & 1                    & 26.2 & 24.9 & 27.1 & 25.6 & 24.4 & 24.7 & 25.5    & 24.4 \\
& & & 0.1                  & 23.0 & 16.0 & 17.4 & 18.3 & 21.1 & 16.1 & 18.7    & 16.0 \\
& & & 0.01                 & 14.4 & 14.5 & 13.9 & 12.1 & 11.2 & 12.4 & 13.1    & 11.2 \\
\cline{3-12}
& & \multirow{5}{*}{\shortstack{Linear\\ Probe}} & 100 & 34.4 & 34.7 & 33.4 & 31.2 & 34.0 & 32.7 & 33.4    & 31.2 \\
& & & 10                   & 35.0 & 31.5 & 32.5 & 33.3 & 32.7 & 32.6 & 32.9    & 31.5 \\
& & & 1                    & 32.5 & 33.7 & 35.3 & 32.8 & 32.9 & 33.0 & 33.4    & 32.5 \\
& & & 0.1                  & 39.7 & 31.3 & 34.6 & 35.8 & 37.0 & 30.9 & 34.9    & 31.3 \\
& & & 0.01                 & 35.0 & 36.8 & 33.7 & 32.5 & 33.7 & 32.4 & 34.0    & 32.4 \\
\cline{2-12}
& \multirow{5}{*}{SimCLR} & \multirow{5}{*}{\shortstack{Linear\\ Probe}} & 100 & 34.0 & 41.7 & 19.2 & 12.4 & 40.6 & 30.6 & 29.8    & 12.4 \\
& & & 10                     & 41.8 & 41.9 & 39.6 & 38.9 & 41.9 & 34.9 & 39.8    & 34.9 \\
& & & 1                      & 41.8 & 42.3 & 43.0 & 43.5 & 42.6 & 42.7 & 42.7    & 41.8 \\
& & & 0.1                    & 45.5 & 24.8 & 41.7 & 40.6 & 43.8 & 40.4 & 39.5    & 24.8 \\
& & & 0.01                   & 44.0 & 42.3 & 42.8 & 43.2 & 41.2 & 42.3 & 42.6    & 41.2 \\
\shline
\multirow{3}{*}{\shortstack{Tiny-\\ImageNet}} & \multirow{3}{*}{SimCLR} & \multirow{3}{*}{\shortstack{Linear\\ Probe}} & 100 & 35.5 & 35.0 & 35.4 & 35.5 & 35.6 & 35.0 & 35.3 & 35.0 \\
& & & 1    & 36.3 & 34.7 & 35.4 & 35.4 & 35.6 & 35.9 & 35.6 & 34.7 \\
& & & 0.01 & 36.2 & 35.6 & 34.6 & 36.1 & 35.3 & 35.8 & 35.6 & 35.3 \\
\shline
\multirow{3}{*}{\shortstack{ImageNet-100}} & \multirow{3}{*}{SimCLR} & \multirow{3}{*}{\shortstack{Linear\\ Probe}} & 100 & 65.0 & 64.9 & 64.2 & 64.5 & 63.7 & 64.8 & 64.5 & 63.7 \\
& & & 1    & 66.2 & 64.5 & 65.6 & 65.3 & 63.2 & 61.5 & 64.4 & 61.5 \\
& & & 0.01 & 61.3 & 59.0 & 64.0 & 61.8 & 59.6 & 64.3 & 61.7 & 59.0
\end{tabular}
\end{center}
\caption{Local training of supervised/self-supervised learning on 4 different datasets with different degrees of non-\iid-ness. Both methods are fully evaluated on CIFAR10/CIFAr100. For Tiny-ImageNet and ImageNet, we provide self-supervised method SimCLR's performances that is used in the main body of our paper.}
\label{tab:cifar10-sl-acc}
\vspace{5em}
\end{table*}

%%%%%%%%%%%%%%%%%% Communication Rounds %%%%%%%%%%%%%
\begin{table*}[p]
\vspace{6em}
\begin{center}
\tablestyle{10pt}{1.35}
\begin{tabular}{c|c|cccccc}
\toprule
& \multirow{2}{*}{Non-\iid-ness $\alpha$} & \multicolumn{6}{c}{Communication Rounds $T$} \\
& & 1    & 2    & 4    & 10   & 20   & 40   \\
\shline
\multirow{3}{*}{FedAvg} & 100  & 6.8  & 21.3 & 34.2 & 37.8 & 36.8 & 36.6 \\
& 1    & 10.9 & 37.0 & 42.5 & 43.2 & 41.5 & 37.2 \\
& 0.01 & 10.3 & 34.2 & 42.5 & 44.8 & 42.4 & 38.4 \\
\hline
\multirow{3}{*}{\ours} & 100  & 18.9 & 36.0 & 39.2 & 35.4 & 36.7 & 34.8 \\
& 1    & 42.1 & 43.8 & 43.0 & 37.9 & 34.4 & 33.4 \\
& 0.01 & 41.4 & 42.2 & 38.8 & 33.3 & 29.4 & 31.6 \\
\bottomrule
\end{tabular}
\end{center}
\vspace{0em}
\caption{Influence of the communication rounds with total epochs set constant $E_\text{total}$=200, evaluated on CIFAR100.}
\label{tab:comm-fix-total}
\end{table*}

%%%%%%%%%%%%%%%%%% Communication Rounds %%%%%%%%%%%%%
\begin{table*}[p]
\begin{center}
\tablestyle{6pt}{1.35}
\begin{tabular}{c|c|cccccccccccc}
\toprule
& \multirow{2}{*}{Non-\iid-ness $\alpha$} & \multicolumn{12}{c}{Communication Rounds $T$} \\
& & 1    & 2    & 3    & 4    & 5    & 6    & 7    & 8    & 9    & 10   & 15   & 20   \\
\shline
\multirow{3}{*}{FedAvg} & 100  & 18.6 & 33.0   & 39.2 & 43.3 & 46.2 & 47.9 & 49.2 & 50   & 50.7 & 51.2 & 51.4 & 52.0   \\
& 1.0    & 36.7 & 45.2 & 48.6 & 50.8 & 51.2 & 51.4 & 51.6 & 51.7 & 51.8 & 52.1 & 52.6 & 52.4 \\
& 0.01 & 32.5 & 42.2 & 46.8 & 47.9 & 48.6 & 48.3 & 48.4 & 48.3 & 48.4 & 48.3 & 48.4 & 48.4 \\
\hline
\multirow{3}{*}{\ours} & 100 & 31.9 & 37.4 & 40.0   & 41.8 & 41.6 & 41.6 & 41.3 & 40.9 & 40.5 & 39.8 & 39.0   & 39.1   \\
& 1 & 40.5 & 43.0   & 44.4 & 45.1 & 44.5 & 44.0   & 43.1 & 42.7 & 42.4 & 41.9 & 40.5 & 39.6   \\
& 0.01 & 40.3 & 42.8 & 43.0   & 42.0   & 41.1 & 40.0   & 38.6 & 38.3 & 37.5 & 36.8 & 35.1 & 34.1  \\
\bottomrule
\end{tabular}
\end{center}
\vspace{0em}
\caption{Influence of the communication rounds with local epochs set constant $E_\text{local}$=100, evaluated on CIFAR100.}
\label{tab:comm-fix-local}
\end{table*}

\begin{table*}[p]
\begin{center}
\tablestyle{10pt}{1.35}
\begin{tabular}{c|c|cccc}
\toprule
& \multirow{2}{*}{Non-\iid-ness $\alpha$} & \multicolumn{4}{c}{Local Epochs $E_\text{local}$} \\
& & 100    & 200    &400    & 800    \\
\shline
\multirow{3}{*}{FedAvg} & 100 & 21.0 & 20.6 & 20.0 & 19.9 \\
& 1    & 37.0 & 40.1 & 24.0 & 4.8 \\
& 0.01 & 34.2 & 31.8 & 11.3 & 1.0 \\
\hline
\multirow{3}{*}{\ours} & 100 & 36.0 & 37.9 & 43.4 & 45.6 \\
& 1    & 43.8 & 47.3 & 47.5 & 47.5 \\
& 0.01 & 42.2 & 43.9 & 42.7 & 39.3\\
\bottomrule
\end{tabular}
\end{center}
\vspace{0em}
\caption{Influence of the local training epochs with communication rounds restricted to $T$=2, evaluated on CIFAR100.}
\label{tab:comm-fix-global}
\vspace{6em}
\end{table*}

%%%%%%%%%%%%%%%%%%%%%%%%%%%%%%%%%%%%%%%%%%%%%%%%%%%%%%%%%%
%%%%%%%%%       Different Components of FLESD
%%%%%%%%%%%%%%%%%%%%%%%%%%%%%%%%%%%%%%%%%%%%%%%%%%%%%%%%%%
\begin{table*}[p]
\begin{center}
\tablestyle{10pt}{1.35}
\begin{tabular}{c|ccccc}
\toprule
\multirow{2}{*}{Non-\iid-ness $\alpha$} & \multicolumn{5}{c}{Percentage of Similarity Matrix Preserved (\%).} \\
& 1\%    & 10\%     & 20\%    & 50\% & 100\%   \\
\shline
100  & 44.2 & 36.7 & 34.6 & 34.4 & 36.0 \\
1    & 44.6 & 43.5 & 44.0 & 43.7 & 43.8 \\
0.01 & 43.7 & 42.0 & 43.3 & 42.8 & 42.2 \\
\bottomrule
\end{tabular}
\end{center}
\vspace{-0.5em}
\caption{FLESD case study on \textbf{Similarity Matrix Quantization}, evaluated on CIFAR100.}
\label{tab:case-quant}
\end{table*}

\begin{table*}[p]
\begin{center}
\tablestyle{10pt}{1.35}
\begin{tabular}{c|cccccc}
\toprule
\multirow{2}{*}{Non-\iid-ness $\alpha$} & \multicolumn{6}{c}{Ensemble Similarity Distillation Temperatures $\tau_T$=$\tau_S$} \\
     & 0.01 & 0.05 & 0.1  & 0.2  & 0.5  & 1.0  \\
\shline
100  & 40.7 & 34.2 & 34.4 & 33.1 & 32.4 & 24.2 \\
1    & 41.6 & 43.3 & 44.0 & 41.7 & 35.8 & 28.7 \\
0.01 & 42.0 & 43.6 & 42.8 & 39.5 & 33.4 & 26.5 \\
\bottomrule
\end{tabular}
\end{center}
\vspace{-0.5em}
\caption{FLESD case study on \textbf{Ensemble Similarity Distillation Temperatures}, evaluated on CIFAR100.}
\label{tab:case-temp}
\end{table*}

\begin{table*}[p]
\begin{center}
\tablestyle{10pt}{1.35}
\begin{tabular}{c|cccccc}
\toprule
\multirow{2}{*}{Non-\iid-ness $\alpha$} & \multicolumn{6}{c}{Anchor Set Size $m$} \\
     & 128  & 256  & 512  & 1024 & 2048 & 4096 \\
\shline
100  & 41.2 & 41.9 & 41.0 & 34.9 & 31.7 & 31.3 \\
1    & 43.5 & 44.0 & 45.2 & 44.8 & 43.4 & 41.8 \\
0.01 & 42.7 & 44.7 & 44.6 & 44.5 & 42.6 & 41.0 \\
\bottomrule
\end{tabular}
\end{center}
\vspace{-0.5em}
\caption{FLESD case study on \textbf{Anchor Set Size $m$}, evaluated on CIFAR100.}
\label{tab:case-anchor}
\end{table*}

\begin{table*}[p]
\begin{center}
\tablestyle{10pt}{1.35}
\begin{tabular}{c|ccccc}
\toprule
\multirow{2}{*}{Non-\iid-ness $\alpha$} & \multicolumn{5}{c}{Momentum Encoder Factor $\zeta$} \\
     & 0    & 0.9  & 0.99 & 0.999 & 0.9999 \\
\shline
100  & 21.7 & 28.0 & 31.2 & 35.1  & 32.2   \\
1    & 35.5 & 35.5 & 42.0 & 44.8  & 43.6   \\
0.01 & 33.1 & 34.9 & 40.4 & 41.7  & 41.9 \\
\bottomrule
\end{tabular}
\end{center}
\vspace{-0.5em}
\caption{FLESD case study on \textbf{Momentum Encoder Factor $\zeta$}, evaluated on CIFAR100.}
\label{tab:case-momentum}
\end{table*}

\begin{table*}[p]
\begin{center}
\tablestyle{10pt}{1.35}
\begin{tabular}{c|cccc}
\toprule
\multirow{2}{*}{Non-\iid-ness $\alpha$} & \multicolumn{4}{c}{Batch Size of \ours} \\
     & 128  & 256  & 512  & 1024 \\
\shline
100  & 39.2 & 39.5 & 38.7 & 37.8 \\
1    & 43.8 & 45.7 & 44.0 & 42.3 \\
0.01 & 42.2 & 42.5 & 38.0 & 37.1 \\
\bottomrule
\end{tabular}
\end{center}
\vspace{-0.5em}
\caption{FLESD case study on \textbf{Batch Size of \ours}, evaluated on CIFAR100.}
\label{tab:case-bs}
\end{table*}
